# Supplementary material for: A Toolkit for Virtual Reality Data Collection
Source: arXiv:2412.17490 source file (2024-12-23)
Supplement: Supplementary file 1 [file GazeDatasetSpecification.pdf]

Universität Hamburg
DER FORSCHUNG | DER LEHRE | DER BILDUNG

# The SPOVR Standard: Specification, Protocols, and Organization of VR Datasets

*Or whatever name fits best*

**Tim Rolff**
University of Hamburg

Universität Hamburg
DER FORSCHUNG | DER LEHRE | DER BILDUNG

Copyright ©2024 University of Hamburg

`www.uni-hamburg.de`

*First edition, December 1, 2024*

CHAPTER 0

# Contents

1 **Introduction** 1

2 **Document Conventions** 3

2.1 Normative Terminology . . . . . 3

2.2 Modalities Terminology . . . . . 4

2.3 Metrics . . . . . 5

2.3.1 Angular Error . . . . . 5

3 **Definitions** 6

3.1 Dataset Terminology . . . . . 6

4 **Challenges** 8

4.1 Eye-Tracking Challenges . . . . . 8

4.1.1 Gaze Prediction . . . . . 8

4.1.2 Gaze Forecasting . . . . . 9

4.1.3 Time-to-Saccade Prediction . . . . . 10

4.1.4 Saliency Prediction . . . . . 10

4.1.5 Multiuser Gaze Prediction . . . . . 10

4.2 Movement Challenges . . . . . 11

4.2.1 Locomotion Prediction . . . . . 11

4.2.2 Head and Body Motion Prediction . . . . . 11

4.3 Input Challenges . . . . . 12

4.3.1 User Input Prediction . . . . . 12

4.3.2 Time-to-Input Prediction . . . . . . . . . . 12
4.4 Questionnaire Challenges . . . . . . . . . . 13
4.4.1 User Experience Prediction . . . . . . . . . . 13
4.4.2 VR Sickness Prediction . . . . . . . . . . 13
4.4.3 Cognitive Workload Prediction . . . . . . . . . . 14
4.5 Computer Vision Challenges . . . . . . . . . . 14
4.5.1 Future Frame Prediction . . . . . . . . . . 14
4.5.2 Depth Estimation . . . . . . . . . . 15
4.5.3 Optical Flow Estimation . . . . . . . . . . 15
4.5.4 Segmentation . . . . . . . . . . 16

**5 Organization** **17**
5.1 Required Data . . . . . . . . . . 17

**6 Implementation & Protocols** **19**
6.1 Data Structure . . . . . . . . . . 19
6.2 Minimal Specification . . . . . . . . . . 19

**References** **21**

# Chapter 1 Introduction

This document provides an overview of the EyeRes dataset collection, its organizational structure, protocols, and specification. This dataset aims for a collection of important data samples for common virtual reality (VR) challenges and problems. It should provide an initial collection that is later extended with additional data. This project aims to provide a new benchmark, challenges and training dataset for egocentric VR prediction challenges. The goal of the project is to provide researchers with a large-scale dataset for deep-learning benchmarks to compare different deep-learning architectures. Therefore, our objective is to collect a dataset large enough for pre-training neural networks, such that it allows for transfer learning onto smaller datasets. Here, pre-training describes the process of training a neural network on a large dataset using a general task as objective, for example in other research domains being equivalent to a word completion or image classification problem. This then allows to transfer the learned weights onto a new dataset with less data using the original or a different objective. A big enough size of the dataset is of most importance as modern deep-learning algorithms easily overfit on small datasets or a specific environment. Therefore, to avoid the network learning the input data by hearth it is essential to provide a big enough dataset of previously unseen data containing the required data modalities.

To provide a sufficiently sized dataset, we will collect data of different VR applications and experiments mainly performed by members or students of the Human Computer Interaction (HCI) or the Computer Vision (CV) group at the University of Hamburg. However, we would also like to allow other researchers or cooperation partners to contribute to this project as this would open possibilities to advance other research directions. Therefore, we want to perform our experiment in parallel with existing and running studies to capture the required amount

of data. Therefore, the data capturing in this project can effectively be seen as an unrelated study which extends the underlying experiment for additional data collection. We will not gather data as secondary use. This also allows us to capture multiple different tasks with visually distinct environments without the requirement to develop multiple applications.

The captured dataset will be used to for multiple open challenges, such as gaze forecasting, gaze event prediction, head or hand movement prediction and observation a complex relationship among fixations, saccades, and other eye-movements. Furthermore, we focus on finding correlations between gaze data and the visual stimulus, head or hand movements, or the interactions with the environment.

CHAPTER 2

# Document Conventions

The specification is intended for use by both implementors of the API and application developers seeking to make use of the API for dataset collection, forming a contract between these parties. Specification text may address either party; typically, the intended audience can be inferred from context, though some sections are defined to address only one of these parties. (For example, Valid Usage sections only address application developers). Any requirements, prohibitions, recommendations, or options defined by normative terminology are imposed only on the audience of that text.

## 2.1 | Normative Terminology

(Shamelessly stolen from the OpenXR documentation)

The key words ***must***, ***required***, ***should***, ***may***, and ***optional*** in this document, when denoted as above, are to be interpreted as described in RFC 2119: tools.ietf.org/html/rfc2119.

***must***

When used alone, this word, or the term ***required***, means that the definition is an absolute requirement of the specification. When followed by not ("***must not***"), the phrase means that the definition is an absolute prohibition of the specification.

***should***

When used alone, this word means that there ***may*** exist valid reasons in particular circumstances to ignore a particular item, but the full implications must be under-

stood and carefully weighed before choosing a different course. When followed by not ("***should not***"), the phrase means that there ***may*** exist valid reasons in particular circumstances when the particular behavior is acceptable or even useful, but the full implications should be understood, and the case carefully weighed before implementing any behavior described with this label.

***may***

This word, or the adjective ***optional***, means that an item is truly ***optional***. One vendor ***may*** choose to include the item because a particular marketplace requires it or because the vendor feels that it enhances the product while another vendor ***may*** omit the same item.

The additional terms ***can*** and ***cannot*** are to be interpreted as follows:

***can***

This word means that the particular behavior described is a valid choice for an application and is never used to refer to runtime behavior.

***cannot***

This word means that the particular behavior described is not achievable by an application, for example, an entry point does not exist.

There is an important distinction between ***cannot*** and ***must not***, as used in this Specification. Cannot means something during data collection that is literally impossible to express or accomplish, while ***must not*** means something that is possible during data collection, but that the consequences of doing so are undefined or not allowed and potentially unrecoverable for future use of the dataset.

## 2.2 | Modalities Terminology

***Gaze Vector***

Lorem ipsum dolor sit amet, consectetuer adipiscing elit. Ut purus elit, vestibulum ut, placerat ac, adipiscing vitae, felis. Curabitur dictum gravida mauris. Nam arcu libero, nonummy eget, consectetuer id, vulputate a, magna. Donec vehicula augue eu neque. Pellentesque habitant morbi tristique senectus et netus et malesuada fames ac turpis egestas. Mauris ut leo. Cras viverra metus rhoncus sem. Nulla et lectus vestibulum urna fringilla ultrices. Phasellus eu tellus sit amet tortor gravida placerat.

Integer sapien est, iaculis in, pretium quis, viverra ac, nunc. Praesent eget sem vel leo ultrices bibendum. Aenean faucibus. Morbi dolor nulla, malesuada eu, pulvinar at, mollis ac, nulla. Curabitur auctor semper nulla. Donec varius orci eget risus. Duis nibh mi, congue eu, accumsan eleifend, sagittis quis, diam. Duis eget orci sit amet orci dignissim rutrum.

***Gaze Events***

Lorem ipsum dolor sit amet, consectetuer adipiscing elit. Ut purus elit, vestibulum ut, placerat ac, adipiscing vitae, felis. Curabitur dictum gravida mauris. Nam arcu libero, nonummy eget, consectetuer id, vulputate a, magna. Donec vehicula augue eu neque. Pellentesque habitant morbi tristique senectus et netus et malesuada fames ac turpis egestas. Mauris ut leo. Cras viverra metus rhoncus sem. Nulla et lectus vestibulum urna fringilla ultrices. Phasellus eu tellus sit amet tortor gravida placerat. Integer sapien est, iaculis in, pretium quis, viverra ac, nunc. Praesent eget sem vel leo ultrices bibendum. Aenean faucibus. Morbi dolor nulla, malesuada eu, pulvinar at, mollis ac, nulla. Curabitur auctor semper nulla. Donec varius orci eget risus. Duis nibh mi, congue eu, accumsan eleifend, sagittis quis, diam. Duis eget orci sit amet orci dignissim rutrum.

## 2.3 | Metrics

### 2.3.1 | Angular Error

Lorem ipsum dolor sit amet, consectetuer adipiscing elit. Ut purus elit, vestibulum ut, placerat ac, adipiscing vitae, felis. Curabitur dictum gravida mauris. Nam arcu libero, nonummy eget, consectetuer id, vulputate a, magna. Donec vehicula augue eu neque. Pellentesque habitant morbi tristique senectus et netus et malesuada fames ac turpis egestas. Mauris ut leo. Cras viverra metus rhoncus sem. Nulla et lectus vestibulum urna fringilla ultrices. Phasellus eu tellus sit amet tortor gravida placerat. Integer sapien est, iaculis in, pretium quis, viverra ac, nunc. Praesent eget sem vel leo ultrices bibendum. Aenean faucibus. Morbi dolor nulla, malesuada eu, pulvinar at, mollis ac, nulla. Curabitur auctor semper nulla. Donec varius orci eget risus. Duis nibh mi, congue eu, accumsan eleifend, sagittis quis, diam. Duis eget orci sit amet orci dignissim rutrum.

CHAPTER 3

# Definitions

## 3.1 | Dataset Terminology

***Timestamp***

Exact time of an event capture in (milliseconds?, microseconds?) using the UNIX POSIX format.

***Sample***

A singular data point capturing a data point of one device that must occur at the exact same time. These may include multiple modalities or values, for example capturing axes or rotation through vectors or quaternions. Furthermore, a sample should include multiple values at once if they can be captured at the same time from the same device. A value is considered captured at the same time only if the queried device returns the values together or with the same timestamp. Whenever possible, a sample must contain the timestamp at which it got captured.

***Examples for valid samples:***

- A vector $(x, y, z)$ and *timestamp* containing the current position of the HMD captured at the same time.
- A vector $(x, y, z)$, quaternion $(x, y, z, w)$ and *timestamp* containing the position, rotation, and time of the capture from the Controller captured at the same time.
- A *timestamp* with a float value and a Boolean containing the openness of the

pupil and the state of a blink, both captured at the same time.

***Examples for invalid samples:***

- A vector $(x, y, z)$ with one timestamp and a quaternion with another *timestamp* containing the position and rotation of the HMD at separate times.

  ***Note:*** This is invalid because it captures values at different time points. These should be considered as two different samples.
- A vector $(x, y, z)$ and a quaternion $(x, y, z, w)$ captured at the same time.

  ***Note:*** This is invalid because it misses the timestamp for a sample that must be included.
- A vector $(x, y, z)$ and *timestamp* containing the position of the HMD with each axis captured at separate times.

  ***Note:*** This is invalid because it captures values of the same vector at different time points.

***Snapshot***

A collection of samples captured during the same frame. The duration of a frame is defined as the start of the display of the rendered image till the next rendered frame.

***Sequence***

A collection of samples captured during a full run of a participant in the virtual environment. To satisfy the definition of a sequence the timestamps of the samples must be in ascending order.

***Trial***

A collection of snapshots and sequences of all modalities capturing during one run for data collection. Note that an experiment can have multiple conditions that each result in their own trial. A trial must not contain pauses that do not capture data from the participant, for example while filling out questionnaires or during the adjustment of the HMD.

***Dataset***

Full collection of all sequences and snapshots captured from all trials.

CHAPTER 4

# Challenges

As VR provides a good opportunity to capture data from different sensors and modalities, we propose the following challenges for our dataset. Hence, the dataset must include data modalities to train and validate on. In the following section, we briefly want to explain the challenges and the required data modalities.

## 4.1 | Eye-Tracking Challenges

### 4.1.1 | Gaze Prediction

Prediction of the gaze where users are currently focusing on. Gaze prediction is defined without an eye-tracker (Hu et al., 2020; Hu et al., 2021) using the other modalities provided by the HMD to predict the current gaze point. This challenge aims to provide HMD without eye-trackers with the ability to estimate the current gaze point without relying on the head gaze. This challenge must not use any gaze points provided but may use any other data modality, such as the IMU of the HMD. Most notable works on this are Hu et al. (2020, 2021).

*Goal* — Predict the gaze vector in local coordinates of the HMD without previous gaze data.

*Input* — All modalities from the past are allowed, except for gaze data. Meaning that models may use any input modality, but are not forced to do so. Further, models must not use data past the current gaze point and are not allowed to use gaze data at all. The past is defined such that it is all input data before the current target in the temporal sequence.

*Evaluation* Most optimal model is the one with the smallest error across all metrics.

- Total angular error between prediction and target
- Average fixation angular error between prediction and target
- Average saccade angular error between prediction and target
- Average saccade landing position angular error between prediction and target

### 4.1.2 | Gaze Forecasting

Forecasting the gaze of participants several milliseconds into the future (Hu et al., 2022). This challenge aims to provide a method for latency reduction when utilizing HMDs with eye-trackers. The challenge may use any data modality provided by the HMD but must not use future gaze points.

*Goal* Predict the future gaze vector in local coordinates of the HMD using previous gaze data. Gaze should be offset by 50ms, 100ms and 150ms for short-term prediction. For long-term prediction, gaze should be offset by 1s, 10s, and 60s.

*Input* All modalities from the past are allowed. The past is defined such that it is all input data x ms before the target in the temporal sequence, where x is the offset to predict. Meaning that models may use any input modality but are not forced to do so. Further, models must not use data past the current predicted gaze point. The past is defined such that it is all input data before the current target in the temporal sequence.

*Evaluation* Most optimal model is the one with the smallest error across all metrics.

- Total angular error between prediction and target
- Average fixation angular error between prediction and target
- Average saccade angular error between prediction and target
- Average saccade landing position angular error between prediction and target

### 4.1.3 | Time-to-Saccade Prediction

Prediction of the time until a gaze event, such as a saccade, fixation, blink Rolff et al. (2022, 2023). This challenge aims to provide a method for early detection of important gaze events for latency reduction or preparation of downstream tasks. The challenge may use any data modality provided by the HMD, but must not use future gaze points or gaze events.

*Goal* Predict the future gaze events, saccades, fixations, or blinks using previous data. For long-term prediction, gaze should be offset by 1s, 10s, and 60s.

*Input* All modalities from the past are allowed. The past is defined such that it is all data of the current temporal input sequence before the target. Meaning that models may use any input modality but are not forced to do so but must not use data past the current predicted gaze point.

*Evaluation* Most optimal model is the one with the smallest error across all metrics.

- Todo no clue

### 4.1.4 | Saliency Prediction

@Tim is this useful? Probably not, since we need the ground truth for comparison. Maybe we can argue that we generate it through our paper (Gaze Mapping for Immersive Virtual Environments Based on Image Retrieval, 2020).

*Goal*

*Input*

*Evaluation*

- Todo no clue

### 4.1.5 | Multiuser Gaze Prediction

@Susanne can you write something about this? Do we want this?

*Goal*

*Input*

*Evaluation*

- Todo no clue

## 4.2 | Movement Challenges

### 4.2.1 | Locomotion Prediction

The goal of this challenge is to predict a users locomotion intent in virtual environments using any data modality. The developed models should be able to anticipate the direction and speed of locomotion a user intends to perform. The goal is to enhance VR interaction by enabling seamless and intuitive control. Locomotion prediction can be used for navigation, improving space utilization, and optimizing VR techniques such as redirected walking.

A subset of this challenge is the prediction of future motion specific to true walking. All datasets containing corresponding data are marked.

| | |
|---|---|
| *Goal* | Prediction of a sequence of positions or 2D velocities lasting at least two seconds. |
| *Input* | All modalities from the past are allowed. |
| *Evaluation* | Most optimal model is the one with the smallest euclidean distance across most timesteps. |

- Todo no clue

### 4.2.2 | Head and Body Motion Prediction

Lorem ipsum dolor sit amet, consectetuer adipiscing elit. Ut purus elit, vestibulum ut, placerat ac, adipiscing vitae, felis. Curabitur dictum gravida mauris. Nam arcu libero, nonummy eget, consectetuer id, vulputate a, magna. Donec vehicula augue eu neque. Pellentesque habitant morbi tristique senectus et netus et malesuada fames ac turpis egestas. Mauris ut leo. Cras viverra metus rhoncus sem. Nulla et lectus vestibulum urna fringilla ultrices. Phasellus eu tellus sit amet tortor gravida placerat. Integer sapien est, iaculis in, pretium quis, viverra ac, nunc. Praesent eget sem vel leo ultrices bibendum. Aenean faucibus. Morbi dolor nulla, malesuada eu, pulvinar at, mollis ac, nulla. Curabitur auctor semper nulla. Donec varius orci eget risus. Duis nibh mi, congue eu, accumsan eleifend, sagittis quis, diam. Duis eget orci sit amet orci dignissim rutrum.

*Goal*
*Input*
*Evaluation*

- Todo no clue

## 4.3 | Input Challenges

### 4.3.1 | User Input Prediction

With multiple actions, a user can take and some of them involving the Midas Touch problem, it would be helpful to classify if an action is intended or what the next action would be. This is especially true for gaze interactions, as it is hard to avert the gaze from a possible interaction target even though an interaction might not have been indented. Here, the challenge is to predict the next action a user can take. As the input space is large depending on the application, we define this challenge as the prediction of the correct button or hardware interaction, as those are quite limited.

*Goal*
*Input*
*Evaluation*

- Todo no clue

### 4.3.2 | Time-to-Input Prediction

Lorem ipsum dolor sit amet, consectetuer adipiscing elit. Ut purus elit, vestibulum ut, placerat ac, adipiscing vitae, felis. Curabitur dictum gravida mauris. Nam arcu libero, nonummy eget, consectetuer id, vulputate a, magna. Donec vehicula augue eu neque. Pellentesque habitant morbi tristique senectus et netus et malesuada fames ac turpis egestas. Mauris ut leo. Cras viverra metus rhoncus sem. Nulla et lectus vestibulum urna fringilla ultrices. Phasellus eu tellus sit amet tortor gravida placerat. Integer sapien est, iaculis in, pretium quis, viverra ac, nunc. Praesent eget sem vel leo ultrices bibendum. Aenean faucibus. Morbi dolor nulla, malesuada eu, pulvinar at, mollis ac, nulla. Curabitur auctor semper nulla. Donec varius orci eget risus. Duis nibh mi, congue eu, accumsan eleifend, sagittis quis, diam. Duis eget orci sit amet orci dignissim rutrum.

*Goal*
*Input*
*Evaluation*

- Todo no clue

## 4.4 | Questionnaire Challenges

### 4.4.1 | User Experience Prediction

Lorem ipsum dolor sit amet, consectetuer adipiscing elit. Ut purus elit, vestibulum ut, placerat ac, adipiscing vitae, felis. Curabitur dictum gravida mauris. Nam arcu libero, nonummy eget, consectetuer id, vulputate a, magna. Donec vehicula augue eu neque. Pellentesque habitant morbi tristique senectus et netus et malesuada fames ac turpis egestas. Mauris ut leo. Cras viverra metus rhoncus sem. Nulla et lectus vestibulum urna fringilla ultrices. Phasellus eu tellus sit amet tortor gravida placerat. Integer sapien est, iaculis in, pretium quis, viverra ac, nunc. Praesent eget sem vel leo ultrices bibendum. Aenean faucibus. Morbi dolor nulla, malesuada eu, pulvinar at, mollis ac, nulla. Curabitur auctor semper nulla. Donec varius orci eget risus. Duis nibh mi, congue eu, accumsan eleifend, sagittis quis, diam. Duis eget orci sit amet orci dignissim rutrum.

*Goal*
*Input*
*Evaluation*

- Todo no clue

### 4.4.2 | VR Sickness Prediction

Lorem ipsum dolor sit amet, consectetuer adipiscing elit. Ut purus elit, vestibulum ut, placerat ac, adipiscing vitae, felis. Curabitur dictum gravida mauris. Nam arcu libero, nonummy eget, consectetuer id, vulputate a, magna. Donec vehicula augue eu neque. Pellentesque habitant morbi tristique senectus et netus et malesuada fames ac turpis egestas. Mauris ut leo. Cras viverra metus rhoncus sem. Nulla et lectus vestibulum urna fringilla ultrices. Phasellus eu tellus sit amet tortor gravida placerat. Integer sapien est, iaculis in, pretium quis, viverra ac, nunc. Praesent eget sem vel leo ultrices bibendum. Aenean faucibus. Morbi dolor nulla,

malesuada eu, pulvinar at, mollis ac, nulla. Curabitur auctor semper nulla. Donec varius orci eget risus. Duis nibh mi, congue eu, accumsan eleifend, sagittis quis, diam. Duis eget orci sit amet orci dignissim rutrum.

*Goal*
*Input*
*Evaluation*

- Todo no clue

### 4.4.3 | Cognitive Workload Prediction

Lorem ipsum dolor sit amet, consectetuer adipiscing elit. Ut purus elit, vestibulum ut, placerat ac, adipiscing vitae, felis. Curabitur dictum gravida mauris. Nam arcu libero, nonummy eget, consectetuer id, vulputate a, magna. Donec vehicula augue eu neque. Pellentesque habitant morbi tristique senectus et netus et malesuada fames ac turpis egestas. Mauris ut leo. Cras viverra metus rhoncus sem. Nulla et lectus vestibulum urna fringilla ultrices. Phasellus eu tellus sit amet tortor gravida placerat. Integer sapien est, iaculis in, pretium quis, viverra ac, nunc. Praesent eget sem vel leo ultrices bibendum. Aenean faucibus. Morbi dolor nulla, malesuada eu, pulvinar at, mollis ac, nulla. Curabitur auctor semper nulla. Donec varius orci eget risus. Duis nibh mi, congue eu, accumsan eleifend, sagittis quis, diam. Duis eget orci sit amet orci dignissim rutrum.

*Goal*
*Input*
*Evaluation*

- Todo no clue

## 4.5 | Computer Vision Challenges

### 4.5.1 | Future Frame Prediction

Lorem ipsum dolor sit amet, consectetuer adipiscing elit. Ut purus elit, vestibulum ut, placerat ac, adipiscing vitae, felis. Curabitur dictum gravida mauris. Nam arcu libero, nonummy eget, consectetuer id, vulputate a, magna. Donec vehicula augue eu neque. Pellentesque habitant morbi tristique senectus et netus et malesuada fames ac turpis egestas. Mauris ut leo.

Cras viverra metus rhoncus sem. Nulla et lectus vestibulum urna fringilla ultrices. Phasellus eu tellus sit amet tortor gravida placerat. Integer sapien est, iaculis in, pretium quis, viverra ac, nunc. Praesent eget sem vel leo ultrices bibendum. Aenean faucibus. Morbi dolor nulla, malesuada eu, pulvinar at, mollis ac, nulla. Curabitur auctor semper nulla. Donec varius orci eget risus. Duis nibh mi, congue eu, accumsan eleifend, sagittis quis, diam. Duis eget orci sit amet orci dignissim rutrum.

*Goal*
*Input*
*Evaluation*

- Todo no clue

## 4.5.2 | Depth Estimation

Lorem ipsum dolor sit amet, consectetuer adipiscing elit. Ut purus elit, vestibulum ut, placerat ac, adipiscing vitae, felis. Curabitur dictum gravida mauris. Nam arcu libero, nonummy eget, consectetuer id, vulputate a, magna. Donec vehicula augue eu neque. Pellentesque habitant morbi tristique senectus et netus et malesuada fames ac turpis egestas. Mauris ut leo. Cras viverra metus rhoncus sem. Nulla et lectus vestibulum urna fringilla ultrices. Phasellus eu tellus sit amet tortor gravida placerat. Integer sapien est, iaculis in, pretium quis, viverra ac, nunc. Praesent eget sem vel leo ultrices bibendum. Aenean faucibus. Morbi dolor nulla, malesuada eu, pulvinar at, mollis ac, nulla. Curabitur auctor semper nulla. Donec varius orci eget risus. Duis nibh mi, congue eu, accumsan eleifend, sagittis quis, diam. Duis eget orci sit amet orci dignissim rutrum.

*Goal*
*Input*
*Evaluation*

- Todo no clue

## 4.5.3 | Optical Flow Estimation

Lorem ipsum dolor sit amet, consectetuer adipiscing elit. Ut purus elit, vestibulum ut, placerat ac, adipiscing vitae, felis. Curabitur dictum gravida mauris. Nam arcu libero, nonummy

eget, consectetuer id, vulputate a, magna. Donec vehicula augue eu neque. Pellentesque habitant morbi tristique senectus et netus et malesuada fames ac turpis egestas. Mauris ut leo. Cras viverra metus rhoncus sem. Nulla et lectus vestibulum urna fringilla ultrices. Phasellus eu tellus sit amet tortor gravida placerat. Integer sapien est, iaculis in, pretium quis, viverra ac, nunc. Praesent eget sem vel leo ultrices bibendum. Aenean faucibus. Morbi dolor nulla, malesuada eu, pulvinar at, mollis ac, nulla. Curabitur auctor semper nulla. Donec varius orci eget risus. Duis nibh mi, congue eu, accumsan eleifend, sagittis quis, diam. Duis eget orci sit amet orci dignissim rutrum.

*Goal*
*Input*
*Evaluation*

■ Todo no clue

### 4.5.4 | Segmentation

Lorem ipsum dolor sit amet, consectetuer adipiscing elit. Ut purus elit, vestibulum ut, placerat ac, adipiscing vitae, felis. Curabitur dictum gravida mauris. Nam arcu libero, nonummy eget, consectetuer id, vulputate a, magna. Donec vehicula augue eu neque. Pellentesque habitant morbi tristique senectus et netus et malesuada fames ac turpis egestas. Mauris ut leo. Cras viverra metus rhoncus sem. Nulla et lectus vestibulum urna fringilla ultrices. Phasellus eu tellus sit amet tortor gravida placerat. Integer sapien est, iaculis in, pretium quis, viverra ac, nunc. Praesent eget sem vel leo ultrices bibendum. Aenean faucibus. Morbi dolor nulla, malesuada eu, pulvinar at, mollis ac, nulla. Curabitur auctor semper nulla. Donec varius orci eget risus. Duis nibh mi, congue eu, accumsan eleifend, sagittis quis, diam. Duis eget orci sit amet orci dignissim rutrum.

*Goal*
*Input*
*Evaluation*

■ Todo no clue

CHAPTER 5

# Organization

## 5.1 | Required Data

The dataset aims to collect general information from VR experiments using data points. It must collect inertial measurement unit (IMU) data from the head-mounted display (HMD) and controllers. Further, each data collection must contain an egocentric view showing what participants saw during the usage of the HMD. Here, we will collect the following data:

Based on the challenges explained in chapter 4, the collection of a data sample must include the following data:

***Identifying data***

***Full name***

Full name of participants. To comply with GCPR regulations we will store this in a separate data set. This data set connects each participant's identity to their respective data. We will use this separate data set to be able to delete their data.

***Demographic data***

***Age (in years)***

Research has shown a correlation between age and the speed of eye-movements. We expect there to be a correlation while interacting with the environment

as well, thus we also want to collect variables, enjoyment, motivation, and physical activity.

***Gender***

For women, research has shown a difference between different eye-movements (Coutrot, et al. 2016). Furthermore, other studies have found a difference when performing attention studies (Chacón-Candia, et al. 2020). To not enforce gender roles or gender biases, we will follow the guidelines by (Spiel und Haimson 2019).

***Experience with VR***

With this, we would like to control the potential novelty effect of VR in our experiments.

***Native Language***

It has been shown that language plays an important role when performing reading studies, as different reading patterns emerge dependent on cultural differences of the language (Marcos, et al. 2013).

***Sensor data***

- Raw data of locomotion
- Raw data of your head- and arm-movements
- Raw controller input of interactions
- A video capturing what you saw in the virtual environment.

***Questionnaires***

- Nasa-TLX
- SUS
- IPQ

CHAPTER 6

# Implementation & Protocols

## 6.1 | Data Structure

## 6.2 | Minimal Specification

In order to have a minimal working dataset, the captured data ***must*** provide the following data points:

- The Demographic data ***must*** including the following:
  - Full name: The full name ***must*** be collected as UTF-8.
  - Age: The age ***must*** be collected as a positive integer in years.
  - Gender: The gender ***must*** be selected from the following options:
    - ☐ Woman
    - ☐ Man
    - ☐ Non-binary
    - ☐ Prefere to not disclose
    - ☐ Prefere to self describe ................................

    ***Note:*** The last option ***must*** provide a text field for participants to enter their gender.
  - Experience with VR
  - Native language

- Questionares:
  - Nasa-TLX: This questionare must be captured after the full ***trial*** . For collection the Nasa-TLX must be as provided by who knows???
  - Experiences in Virtual Worlds: The questionaire ***must*** be provided as follows:
  - Simulator Sickness Questionaire:

CHAPTER 7

# References


Zhiming Hu, Sheng Li, Congyi Zhang, Kangrui Yi, Guoping Wang, and Dinesh Manocha. Dgaze: Cnn-based gaze prediction in dynamic scenes. *IEEE transactions on visualization and computer graphics*, 26(5):1902–1911, 2020.

Zhiming Hu, Andreas Bulling, Sheng Li, and Guoping Wang. Fixationnet: Forecasting eye fixations in task-oriented virtual environments. *IEEE Transactions on Visualization and Computer Graphics*, 27(5):2681–2690, 2021.

Tim Rolff, Frank Steinicke, and Simone Frintrop. When do saccades begin? prediction of saccades as a time-to-event problem. In *2022 Symposium on Eye Tracking Research and Applications*, pages 1–7, 2022.

Tim Rolff, Susanne Schmidt, Frank Steinicke, and Simone Frintrop. A deep learning architecture for egocentric time-to-saccade prediction using weibull mixture-models and historic priors. In *Proceedings of the 2023 Symposium on Eye Tracking Research and Applications*, pages 1–8, 2023.
